# Supplementary material for: BigCodec: Pushing the Limits of Low-Bitrate Neural Speech Codec
Source: arXiv:2409.05377 source file (2024-09-09)
Supplement: Supplementary file 1 [file appendix.tex]

\section{Architecture details}
\label{appendix:architecture}

\section{Details of the baselines}
\label{appendix:baseline_details}

\section{Further comparison with other previous works}
\label{appendix:futher_comparison}

\section{Bitrate studies}
\label{appendix:bitrate_comparison}

\section{Other results on out-of-domain data}
\label{appendix:ood_results}
